# Supplementary material for: IMU-HOI: A Symbiotic Framework for Coherent Human-Object Interaction and Motion Capture via Contact-Conscious Inertial Fusion
Source: arXiv:2606.28604 source file (2026-06-26)
Supplement: Supplementary file 1 [file X_suppl.tex]

\clearpage
\setcounter{page}{1}
\maketitlesupplementary

% \section{Rationale}
% \label{sec:rationale}
% % 
% Having the supplementary compiled together with the main paper means that:
% % 
% \begin{itemize}
% \item The supplementary can back-reference sections of the main paper, for example, we can refer to \cref{sec:intro};
% \item The main paper can forward reference sub-sections within the supplementary explicitly (e.g. referring to a particular experiment); 
% \item When submitted to arXiv, the supplementary will already included at the end of the paper.
% \end{itemize}
% % 
% To split the supplementary pages from the main paper, you can use \href{https://support.apple.com/en-ca/guide/preview/prvw11793/mac#:~:text=Delete%20a%20page%20from%20a,or%20choose%20Edit%20%3E%20Delete).}{Preview (on macOS)}, \href{https://www.adobe.com/acrobat/how-to/delete-pages-from-pdf.html#:~:text=Choose%20%E2%80%9CTools%E2%80%9D%20%3E%20%E2%80%9COrganize,or%20pages%20from%20the%20file.}{Adobe Acrobat} (on all OSs), as well as \href{https://superuser.com/questions/517986/is-it-possible-to-delete-some-pages-of-a-pdf-document}{command line tools}.

\makeatletter
% \renewcommand{\@thesubsection}{\thesubsection.\hspace{0.5em}}
% \makeatother

This supplementary document provides additional details to support the main paper. 
Section~\ref{sec:implementation} elaborates on the network architecture and training losses .  
Section~\ref{sec:datasets} summarizes the datasets, evaluation protocols, and baseline implementations. 
Section~\ref{sec:add_analysis} presents extended ablation studies and visualizations, including error distribution analysis and results on real-world sequences. 
Finally, Section~\ref{sec:discussion} discusses limitations and potential future work.

\section{Implementation Details}
\label{sec:implementation}
\noindent\textbf{1) Stage~I: Temperature-controlled contact prior and fusion.}
The Stage~I contact head outputs unnormalized logits 
$\mathbf{z}_t\in\mathbb{R}^2$ for left- and right-hand contact at each time step $t$. 
We first convert them to marginal contact probabilities via a sigmoid,
\[
p_L(t) = \sigma(z_{t,1}),\qquad
p_R(t) = \sigma(z_{t,2}),
\]
and construct the 3-way contact prior over $\{L,R,0\}$ as
\begin{equation}
\boldsymbol{\pi}_t = \big[p_L(t),\ p_R(t),\ 1-\max(p_L(t),p_R(t))\big]\in\Delta^2 ,
\end{equation}
which preserves probability mass when there is no contact and avoids double-counting 
during transitions or bimanual touches. The contact head is implemented as a 
two-layer unidirectional LSTM (hidden size 128, dropout 0.2) followed by a linear layer.

To address the strong imbalance between no-contact and contact frames, 
we train the contact head with focal cross-entropy,
\begin{equation}
\mathcal{L}_{\text{hands}}
= \sum_t\sum_{k\in\{L,R,0\}}
-\alpha_k (1-q_{t,k})^{\gamma}\,y_{t,k}\log q_{t,k},
\end{equation}
where $q_{t,k}$ is the predicted probability of class $k$ after softmax, $y_{t,k}$ is the 
one-hot label, $\gamma=2$ is the focusing parameter, and $\alpha_k$ are 
class weights proportional to the inverse class frequency. 
The object-velocity head is trained jointly using an $\ell_2$ regression loss
on $\hat{\mathbf v}_O(t)$ and a short-horizon integral consistency term as described in the main paper.

\medskip\noindent\emph{Temperature scaling for contact calibration.}
After training the Stage~I module, we apply post-hoc temperature scaling to calibrate 
the contact probabilities. Concretely, we freeze all network parameters and optimize 
a single scalar temperature $\tau_{\mathrm{c}}>0$ on a held-out validation split 
by minimizing the negative log-likelihood
\begin{equation}
\min_{\tau_{\mathrm{c}}}
\ \sum_t -\log q^{\ast}_{t,y_t},
\qquad
q^\ast_t = \mathrm{softmax}\big(\mathbf{z}_t/\tau_{\mathrm{c}}\big),
\end{equation}
where $y_t\in\{L,R,0\}$ is the ground-truth contact label. 
The resulting $\tau_{\mathrm{c}}$ is fixed for all experiments. 
At test time, we replace $q_t$ by $q^\ast_t$ and recompute
$\boldsymbol{\pi}_t$ using the same mapping as above.
This reduces over-confident spikes and yields a contact prior that better matches 
empirical frequencies.

\medskip\noindent\emph{Regularization and temperature-controlled fusion.}
During joint training with the object translation module, we further add a light 
Kullback--Leibler regularizer
\begin{equation}
\mathcal{L}_{\text{cal}} 
= \lambda_{\text{cal}} \sum_t \mathrm{KL}\big(\tilde{\boldsymbol{\pi}}\ \|\ \boldsymbol{\pi}_t\big),
\end{equation}
where $\tilde{\boldsymbol{\pi}}$ is a smoothed empirical prior 
computed from the training set, and $\lambda_{\text{cal}}\ll 1$.
This term discourages extremely peaky predictions while still allowing confident
contact decisions when strongly supported by IMU evidence.

In Stage~III, the calibrated $\boldsymbol{\pi}_t$ serves as a prior over the three 
object-translation branches: left-hand FK, right-hand FK, and object-IMU integration. 
Let $\mathbf g_t\in\mathbb{R}^3$ denote the branch logits produced by a small 
recurrent gating network from contact probabilities, object velocity, and 
object-IMU features. We combine the data-driven scores and the prior as
\begin{equation}
\tilde{\mathbf g}_t = \mathbf g_t + \beta\log\big(\boldsymbol{\pi}_t + \varepsilon\big),
\qquad
\mathbf w_t = \mathrm{softmax}\!\big(\tilde{\mathbf g}_t / \tau_{\mathrm{g}}\big),
\end{equation}
where $\beta$ is a scalar controlling the strength of the prior, 
$\tau_{\mathrm{g}}$ is a gating temperature, $\varepsilon=10^{-6}$ for numerical stability,
and $\mathbf w_t\in\Delta^2$ are the final fusion weights over the three branches. 
We also implement an optional test-time smoothing that linearly blends consecutive
$\mathbf w_t$ and limits their frame-to-frame change, preventing abrupt switching 
between branches. The final object position is obtained by a convex combination of
the left-FK, right-FK and IMU-integrated trajectories using $\mathbf w_t$.

    % wider Methods column for this table
\begin{table*}[t]
\centering
\caption{Additional ablations on IMU-HOI. Numbers are lower-is-better. Best in \textbf{bold}.}
\vspace{-3mm}
\label{tab:additional_ablation}
\setlength{\tabcolsep}{2pt}

\scriptsize
\resizebox{\linewidth}{!}{%
\begin{tabular}{L*{18}{C}}
\toprule
& \multicolumn{6}{c}{OMOMO}
& \multicolumn{6}{c}{$IMHD^{2}$}
& \multicolumn{6}{c}{BEHAVE} \\
\cmidrule(lr){2-7}\cmidrule(lr){8-13}\cmidrule(lr){14-19}
\textbf{Methods}
& Obj Err & HOI Err & Ang Err  & Pos Err & Trans Err & Jitter 
& Obj Err & HOI Err & Ang Err  & Pos Err & Trans Err & Jitter 
& Obj Err & HOI Err & Ang Err  & Pos Err & Trans Err & Jitter  \\
\midrule
\textcircled{1} merged dataset &
12.22 & 16.55 & 8.99 & 2.26 & 10.11 & 2.64 &
51.86 & 54.68 & 13.95 & 3.37 & 13.04 & 10.16 &
18.92 & 22.98 & 9.51 & 2.66 & 10.13 & 7.98 \\
\textcircled{2} w/o joint-train stage &
13.17 & 17.97 & 8.96 & 2.22 & 10.26 & 2.62 &
49.10 & 50.95 & 13.99 & 3.76 & 20.79 & 10.09 &
24.56 & 27.94 & 9.51 & 2.70 & 10.79 & 7.88 \\
\textcircled{3} TransPose-style input &
13.20 & 18.73 & 9.04 & 2.32 & 11.27 & 2.67 &
62.06 & 66.54 & 13.79 & 3.52 & 19.94 & 10.15 &
23.83 & 28.26 & 9.26 & 2.65 & 11.27 & 7.77 \\
\bottomrule
\end{tabular}%
}
\vspace{-0.5em}
\end{table*}

\medskip\noindent\textbf{2) Stage~II: Human loss terms.}
Stage~II predicts a reduced global pose, part-wise joint velocities, local and global
root velocities, integrated root translation, and world-space wrist positions.
Let $\hat{\theta}_t$ and $\theta_t$ denote the predicted and ground-truth SMPL pose,
$\hat{\mathbf{J}}_t$ and $\mathbf{J}_t$ the corresponding joint positions, and
$\hat{\mathbf v}_{\text{part}}(t)$, $\mathbf v_{\text{part}}(t)$ the part-wise 
pseudo-velocities obtained as in DynaIP. We supervise the Stage~II human module 
with the following losses.

\medskip\noindent\emph{Reduced pose loss.}
We follow DynaIP and predict a reduced set of SMPL joint rotations in 6D representation. 
Let $\hat{\mathbf R}^{\text{red}}_t(j)$ and $\mathbf R^{\text{red}}_t(j)$ be the predicted and 
ground-truth rotations for joint $j$ in the reduced set $\mathcal{J}_{\text{red}}$.
The pose loss is
\begin{equation}
\mathcal{L}_{\text{pose}}
= \frac{1}{T|\mathcal{J}_{\text{red}}|}
\sum_{t=1}^{T}
\sum_{j\in\mathcal{J}_{\text{red}}}
\big\|\hat{\mathbf R}^{\text{red}}_t(j)-\mathbf R^{\text{red}}_t(j)\big\|_2^2,
\end{equation}
which in implementation corresponds to an MSE loss between predicted and 
ground-truth 6D rotations.

\medskip\noindent\emph{Part-wise velocity loss.}
The DynaIP-style SubPosers output pseudo-velocities for lower limbs, trunk, 
and upper limbs. Let $\hat{\mathbf v}_{\text{part}}(t)$ and 
$\mathbf v_{\text{part}}(t)$ denote the stacked velocities of the selected joints
in these regions. We penalize their discrepancy with
\begin{equation}
\mathcal{L}_{\text{vel-part}}
= \frac{1}{T}\sum_{t=1}^{T}
\big\|\hat{\mathbf v}_{\text{part}}(t)-\mathbf v_{\text{part}}(t)\big\|_2^2,
\end{equation}
which corresponds to the \texttt{vel\_root} term in our implementation.

\medskip\noindent\emph{Root-velocity and translation losses.}
The two-branch translation head predicts (i) local root velocity from the trunk-velocity
branch, (ii) world-space root velocity after fusing the two branches, and 
(iii) the integrated root translation trajectory. Denote by 
$\hat{\mathbf v}^{\text{loc}}_{\text{root}}(t)$ and 
$\mathbf v^{\text{loc}}_{\text{root}}(t)$ the predicted and ground-truth local root
velocities, by $\hat{\mathbf v}_{\text{root}}(t)$ and $\mathbf v_{\text{root}}(t)$
the world-space root velocities, and by 
$\hat{\mathbf p}_{\text{root}}(t)$ and $\mathbf p_{\text{root}}(t)$ 
the integrated root translations. We use simple $\ell_2$ penalties:
\begin{align}
\mathcal{L}_{\text{root-loc}}
&= \frac{1}{T}\sum_{t=1}^{T}
\big\|\hat{\mathbf v}^{\text{loc}}_{\text{root}}(t)-\mathbf v^{\text{loc}}_{\text{root}}(t)\big\|_2^2,\\
\mathcal{L}_{\text{root-vel}}
&= \frac{1}{T}\sum_{t=1}^{T}
\big\|\hat{\mathbf v}_{\text{root}}(t)-\mathbf v_{\text{root}}(t)\big\|_2^2,\\
\mathcal{L}_{\text{root-trans}}
&= \frac{1}{T}\sum_{t=1}^{T}
\big\|\hat{\mathbf p}_{\text{root}}(t)-\mathbf p_{\text{root}}(t)\big\|_2^2.
\end{align}

\medskip\noindent\emph{Wrist position loss.}
Finally, to stabilize the hand trajectories that will be consumed by Stage~III, 
we supervise the world-space wrist positions. Let 
$\hat{\mathbf p}^{(L)}_H(t),\hat{\mathbf p}^{(R)}_H(t)$ and 
$\mathbf p^{(L)}_H(t),\mathbf p^{(R)}_H(t)$ denote the predicted and ground-truth 
left/right wrist positions. The hand loss is
\begin{equation}
\mathcal{L}_{\text{hand}}
= \frac{1}{2T}\sum_{t=1}^{T} 
\big(
\|\hat{\mathbf p}^{(L)}_H(t)-\mathbf p^{(L)}_H(t)\|_2^2
+
\|\hat{\mathbf p}^{(R)}_H(t)-\mathbf p^{(R)}_H(t)\|_2^2
\big),
\end{equation}
which corresponds to the \texttt{hand\_pos} term.

\medskip\noindent\emph{Overall human loss.}
The total Stage~II human loss is a weighted sum of the above terms:
\begin{equation}
\begin{aligned}
\mathcal{L}_{\text{human}}
&= \lambda_{\text{pose}}\mathcal{L}_{\text{pose}}
+ \lambda_{\text{vel}}\mathcal{L}_{\text{vel-part}} 
+ \lambda_{\text{loc}}\mathcal{L}_{\text{root-loc}}\\
&+ \lambda_{\text{rv}}\mathcal{L}_{\text{root-vel}}
+ \lambda_{\text{rt}}\mathcal{L}_{\text{root-trans}}
+ \lambda_{\text{hand}}\mathcal{L}_{\text{hand}},
\end{aligned}
\end{equation}
where the weighting coefficients $\lambda_{\bullet}$ are kept fixed across all 
experiments and are chosen once on a validation split.

\section{Datasets, Metrics, and Baselines}
\label{sec:datasets}

\paragraph{Datasets.}
We evaluate on three public HOI datasets that differ in capture modality, object diversity, and sequence duration.

\textbf{OMOMO}~\cite{li2023omghm} This set focuses on full-body manipulation of large objects, with roughly $\sim$10 hours of interactions spanning about 15 object categories. Clips are typically short ($\approx$5\,s) and recorded at 30\,fps, featuring actions such as \emph{lift, carry, push, pull, place}.

\textbf{BEHAVE}~\cite{bhatnagar2022behave} Multi-view RGB-D capture of humans interacting with everyday items; 8 subjects and $\sim$20 object categories with diverse everyday actions (e.g., \emph{sitting on, picking up, carrying, pushing/pulling, placing}). The official frame rate is 30\,fps.

$\mathbf{IMHD^{2}}$~\cite{zhao2024imhoi} Video–inertial HOI benchmark at 60\,fps with 10 object categories and rich interaction verbs (\emph{hold, carry, lift, putdown, push, pull, swing, throw/catch}, etc.). Sequences are typically long (often $\ge$60\,s).

\emph{Preprocessing.}
To match temporal statistics, we downsample $IMHD^{2}$ from 60\,fps to 30\,fps. Because $IMHD^{2}$ and BEHAVE contain many $\ge$60\,s sequences while OMOMO clips are around 5\,s, we randomly crop $IMHD^{2}$/BEHAVE into 5–10\,s windows during training and evaluation for balanced sequence lengths.Unless otherwise stated, we adopt an 80/20 train/test split on each dataset at the \emph{sequence} level.For $IMHD^{2}$/BEHAVE, long clips are cropped into 5–10\,s windows \emph{after} the split to avoid leakage. 

\begin{figure*}[t]
    \centering
    % TODO: replace ``fig_additional_qual'' with the actual file name.
    \includegraphics[width=\linewidth]{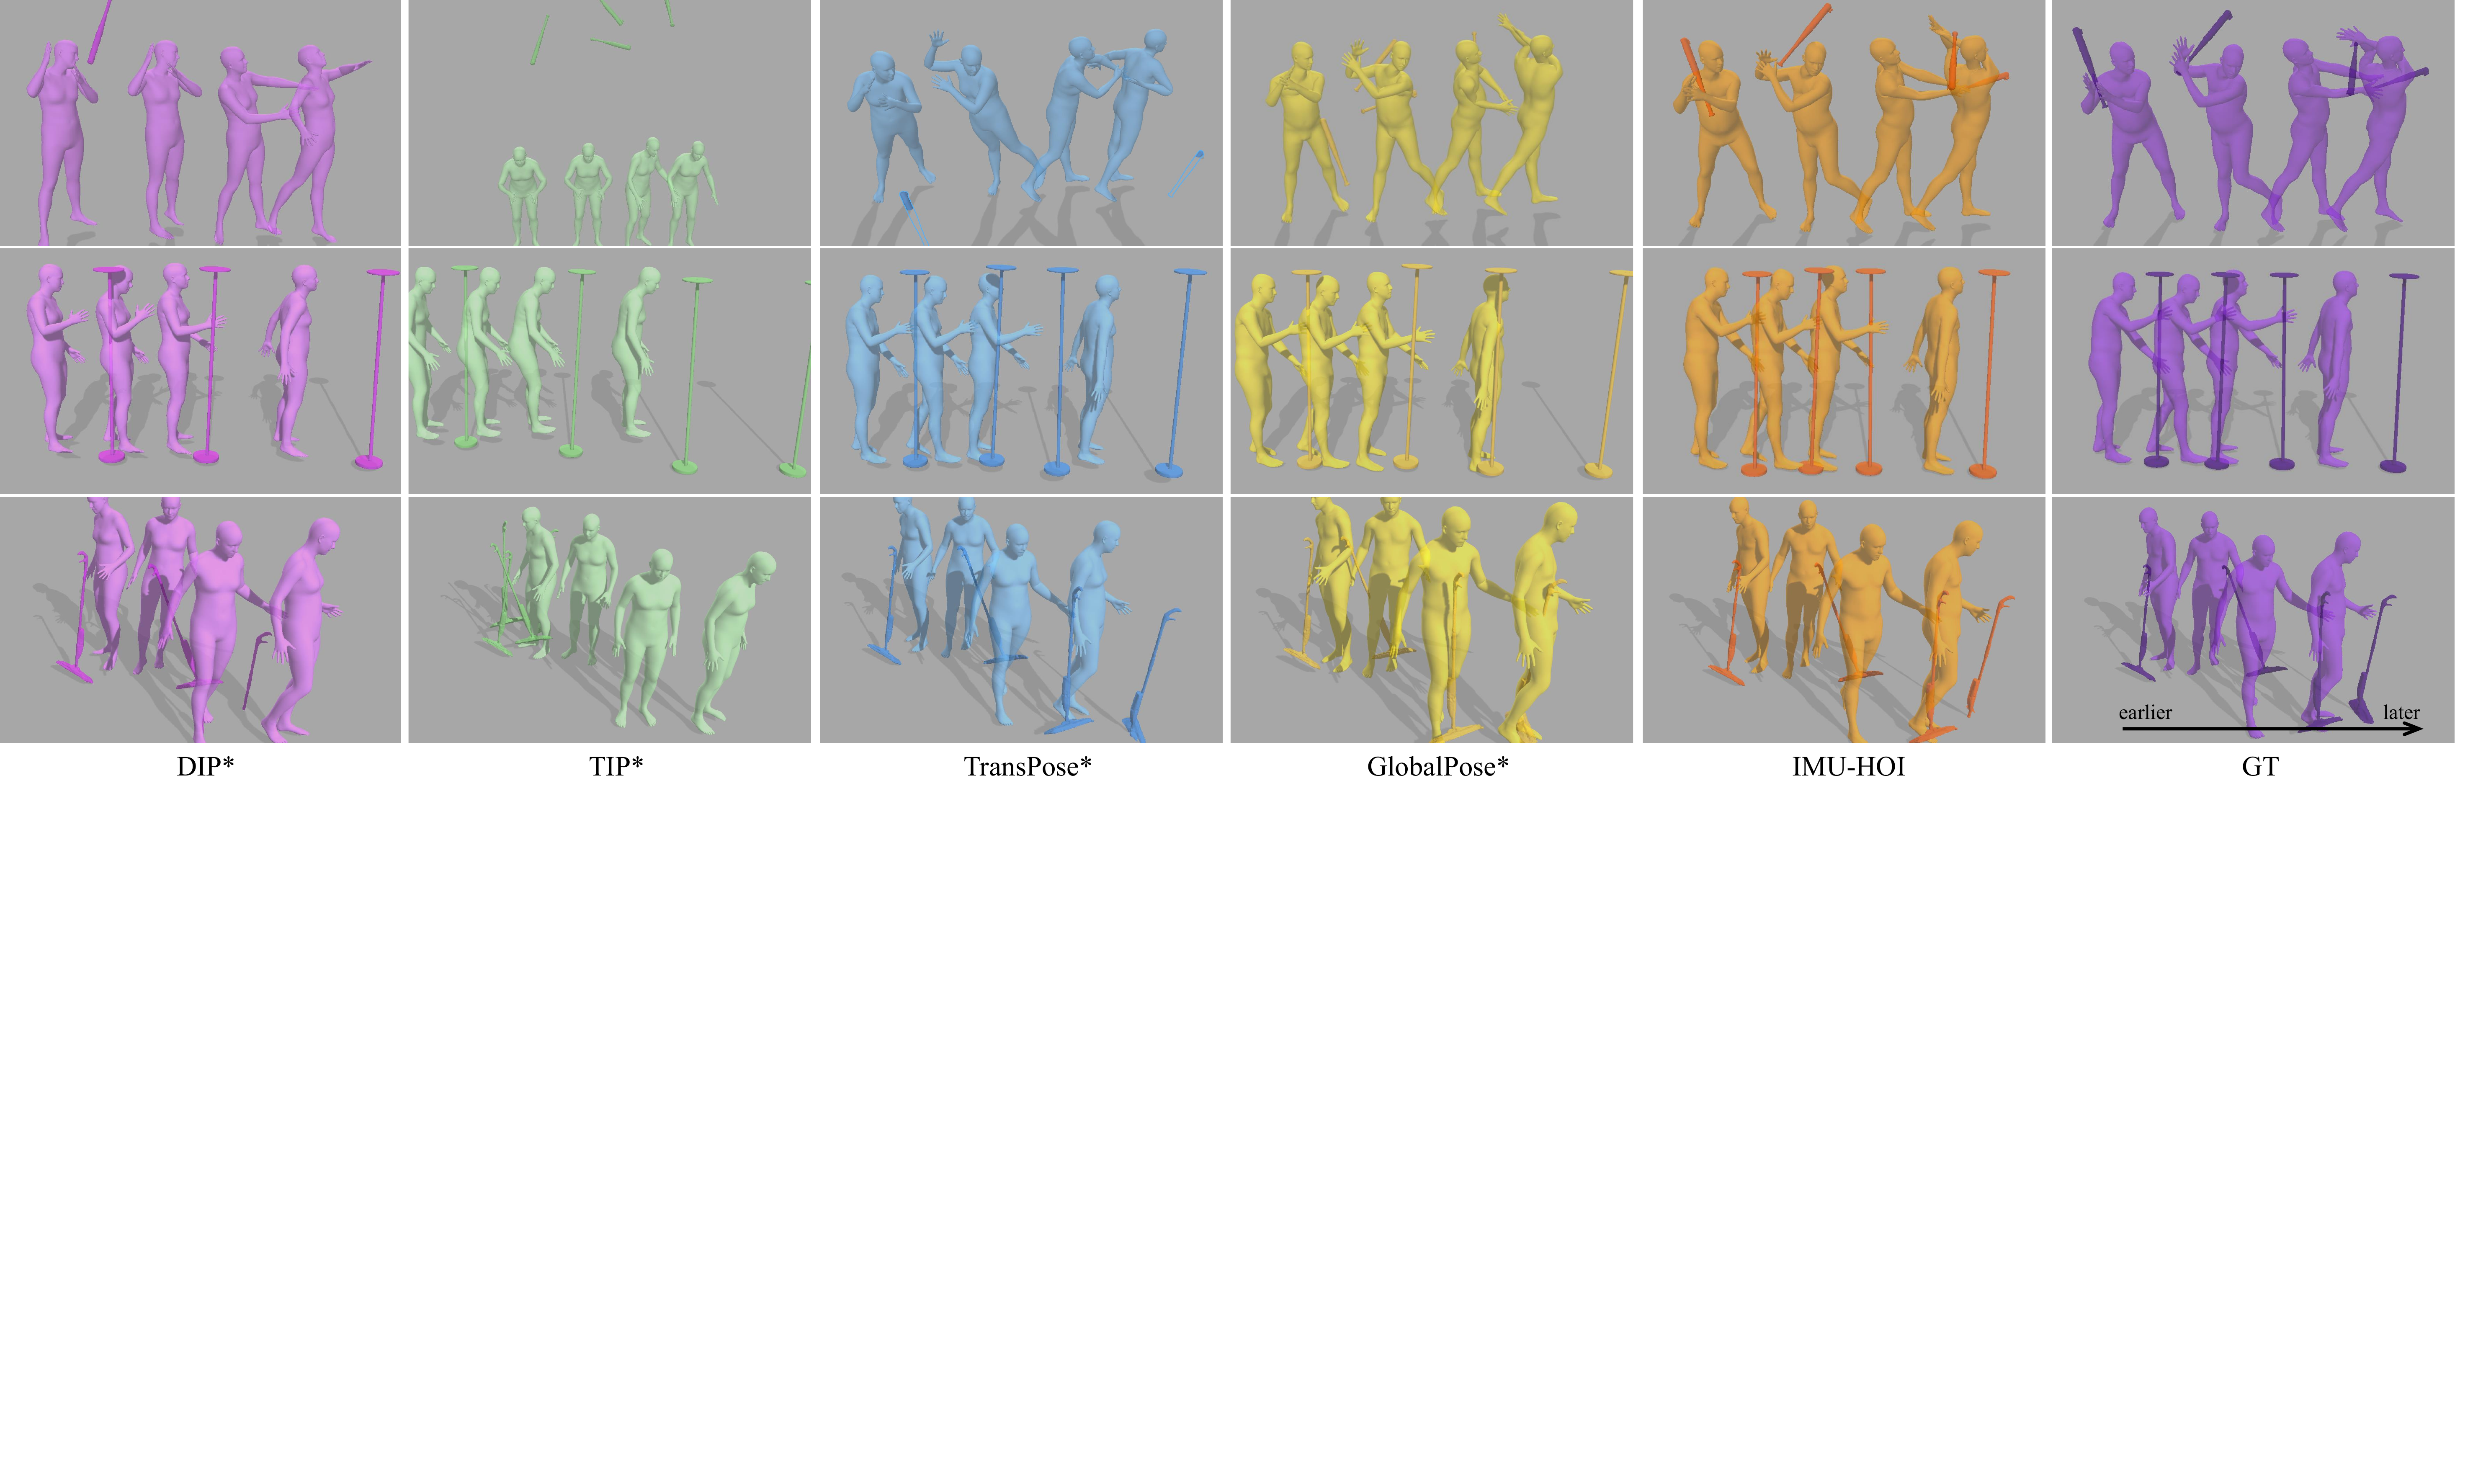}
    \caption{\textbf{Additional qualitative results on OMOMO and IMHD$^2$.}
    For each method we visualize several keyframes of the reconstructed
    human–object interaction.  Baseline methods often exhibit drift in global
    translation, misaligned hand–object contacts, and unstable object
    trajectories.  In contrast, IMU-HOI produces more accurate global motion,
    tighter hand–object contact, and smoother object motion that better
    matches the ground-truth sequence.}
    \label{fig:additional_qual}
\end{figure*}

\paragraph{Competing methods.}
We compare against four strong IMU-based HPE baselines:
\emph{DIP}~\cite{huang2018deep}(recurrent network for pose from sparse IMUs),
\emph{TIP}~\cite{jiang2022transformer}(transformer-based IMU poser),
\emph{TransPose}~\cite{yi2021transpose}(enhanced temporal modeling for sparse-IMU HPE),
and \emph{GlobalPose}~\cite{globalpose_2025} (sparse-IMU HPE augmented with physics-based global motion estimation).
For a fair HOI comparison, we adopt two variants for each: (i) a dimension-augmented baseline that adds an object-IMU branch and an object-velocity head (integrated to object translation), and (ii) the same backbone used as the human module within our contact-gated fusion pipeline. All methods take six body IMUs and one object IMU as input, and share identical splits and evaluation protocols.

\paragraph{Metrics.}
Following prior work~\cite{yi2021transpose,petrov2023object}, we report the following metrics:
\emph{1) Ang Err} [$^\circ$]: the mean global rotation error of all body joints (in degrees);
\emph{2) Pos Err} [cm]: the mean Euclidean distance of all estimated joints with the root joint (Spine) aligned;
\emph{3) Jitter} [mm/s$^3$]: motion smoothness measured by the average \emph{jerk} (rate of change of acceleration) across all joints, where lower is smoother;
\emph{4) Trans Err} [cm]: the average global translation error of the root joint (Spine);
\emph{5) Obj Trans Err} [cm]: the $\ell_2$ distance between the predicted and ground-truth object mesh centers;
\emph{6) HOI Err} [cm] (ours): a \emph{specially} designed interaction metric that evaluates the accuracy of the \emph{relative} hand–object spatial relationship and is computed only on frames with ground-truth hand–object contact. Let $\mathbf{c}^{gt}_t$ and $\hat{\mathbf{c}}_t$ be the GT and predicted object centers, and $\mathbf{h}^{gt}_t$ and $\hat{\mathbf{h}}_t$ the GT and predicted contact-hand joints; with $\mathcal{C}$ the set of GT contact frames, we define
\[
\text{HOI Err}=\frac{1}{|\mathcal{C}|}\sum_{t\in\mathcal{C}}
\big\|(\hat{\mathbf{h}}_t-\hat{\mathbf{c}}_t)-(\mathbf{h}^{gt}_t-\mathbf{c}^{gt}_t)\big\|_2 ,
\]
which emphasizes the accuracy of the hand–object spatial relationship during interaction.

\section{Additional Analysis and Qualitative Results}
\label{sec:add_analysis}

\noindent\textbf{Runtime Comparison.}
To evaluate the computational cost of different methods, we run the released evaluation code of all methods on the three benchmarks and measure the wall-clock evaluation time on a single GPU with a batch size of 1. The reported runtime is the average time (in seconds) required to process the test split of each dataset, with lower numbers indicating faster evaluation. The results are summarized in Tab.~\ref{tab:runtime}. As shown in Tab.~\ref{tab:runtime}, GlobalPose* is by far the slowest method due to its optimization-based pipeline, which requires substantial computational overhead. In comparison, our fusion network introduces moderate additional cost relative to TransPose*, TIP*, and DIP*, but still maintains practical evaluation times across all three datasets. This is acceptable given the substantial accuracy gains achieved by explicitly incorporating human–object interaction reasoning.

\begin{table}[t]
    \centering
    \small
    \setlength{\tabcolsep}{6pt}
    \begin{tabular}{lccc}
        \toprule
        Method & OMOMO & IMHD$^2$ & BEHAVE \\
        \midrule
        TransPose*           & 50.47  & 6.11   & 18.84 \\
        TIP*                 & 54.62  & 5.71   & 18.75 \\
        DIP*                 & 56.73  & 6.01   & 19.92 \\
        GlobalPose*          & 2610.72& 244.08 & 983.53 \\
        Our Method -- Fusion & 134.00 & 15.05  & 46.23 \\
        \bottomrule
    \end{tabular}
    \caption{\textbf{Runtime comparison on the three benchmarks.}
    We report average evaluation time in seconds (lower is better)
    for the trained models.  IMU-only baselines such as TransPose*, TIP*
    and DIP* are very lightweight, whereas the optimization-heavy
    GlobalPose* is two orders of magnitude slower.  Our fusion model is
    roughly $2$--$3\times$ slower than purely kinematic baselines but
    remains dramatically faster than GlobalPose*, while providing
    substantially better HOI reconstruction (see main paper).}
    \vspace{-3mm}
    \label{tab:runtime}
\end{table}

% -------------------------------------------------------------------------

\noindent\textbf{Ablations on Training Strategy and Root Translation.}
We further conduct three ablation studies on our IMU-HOI pipeline to understand the impact of different training strategies and architectural choices:

\begin{itemize}
    \item \textbf{IMU-HOI (joint-all).} This variant is trained using the union of the training and test splits from OMOMO, IMHD$^2$, and BEHAVE, i.e., utilizing all available sequences from the three datasets. This setting serves as an approximate upper bound on the achievable performance of our architecture when more supervision is available.
    
    \item \textbf{IMU-HOI (w/o joint-train stage).} This variant removes the fourth stage of our curriculum, which involves the final joint fine-tuning of Stage~II–III. In this case, each stage is trained separately with its own supervision, and the parameters are frozen when passed to the next stage. This ablation tests the importance of the joint fine-tuning process.
    
    \item \textbf{IMU-HOI-v2 (TransPose-style input).} This variant replaces our velocity-based root-translation head with a TransPose-style design: the B1 branch takes foot joint positions as input, and the B2 branch takes full-body joint positions, rather than the lower-limb and trunk velocity descriptors used in the main method.
\end{itemize}

Tab.~\ref{tab:additional_ablation} reports object translation error, HOI error, body-pose error (Ang/Pos), root translation error, and jitter for all three variants.

On OMOMO and BEHAVE, \emph{IMU-HOI (joint-all)} achieves the best performance across most metrics, suggesting that our architecture can effectively leverage more diverse supervision when trained on the union of the three datasets. Removing the joint fine-tuning stage (\emph{IMU-HOI (w/o joint stage)}) consistently increases HOI error and root-translation error, particularly on BEHAVE, confirming the importance of the final stage for propagating HOI supervision to earlier modules. Replacing our velocity-based root module with a TransPose-style position-based design (\emph{IMU-HOI-v2}) further degrades performance, especially on IMHD$^2$ and BEHAVE, where both HOI error and object translation error increase significantly. These results emphasize the benefits of (i) our staged joint training process and (ii) the contact-aware, velocity-driven root translation head used in the main method.

% -------------------------------------------------------------------------

\noindent\textbf{Additional Qualitative Comparisons.}
Finally, we provide additional qualitative visualizations on OMOMO and IMHD$^2$ comparing IMU-HOI with baseline methods (Fig.~\ref{fig:additional_qual}) . For each sequence, we show a short temporal snippet with several keyframes from the following methods: DIP*, TIP*, TransPose*, GlobalPose*, IMU-HOI, and the ground truth. These visualizations highlight the strengths of our approach in maintaining stable human–object interactions over time, even in the presence of drift and occlusions. Compared to the baselines, IMU-HOI better preserves the hand–object spatial relationship and reduces errors in object trajectory estimation, particularly during long-term interactions. The supplementary visualizations demonstrate the robustness and accuracy of our method in practical, real-world scenarios.

\section{System IMU Deployment and Initialization}
\label{sec:imu_setup}

Before data acquisition, six body-mounted IMUs are attached to the subject at the head, pelvis, both hands, and both feet, respectively, and their mounting orientations are recorded. In addition, one IMU is attached to the manipulated object, with both its mounting position and orientation documented. At the beginning of each recording session, the object is placed between the subject’s two feet under a predefined canonical orientation; for example, the object-IMU local $x$-axis points toward the subject’s left side, the $y$-axis points upward, and the $z$-axis points forward. Before the actual motion recording starts, the subject is required to assume a standard T-pose and remain stationary for $3$--$5$ seconds, during which all IMUs are kept static to estimate their initial rotations for subsequent normalization. Meanwhile, the initial position of the object IMU can be determined from the object dimensions under the predefined placement configuration. During visualization, the object mesh is aligned with the recorded IMU mounting location, so that the estimated object motion can be consistently transferred to the mesh representation.

\begin{figure}[t]
    \centering
    \begin{subfigure}{\columnwidth}
        \centering
        \includegraphics[width=\linewidth]{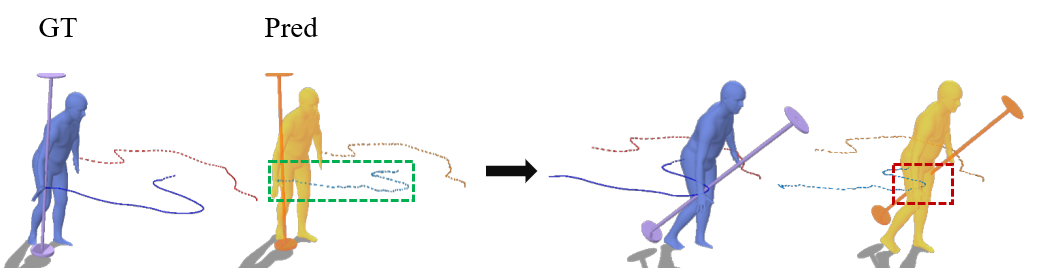}
        \caption{Missed contact}
        \label{fig:failure_case_a}
    \end{subfigure}
    
    \begin{subfigure}{\columnwidth}
        \centering
        \includegraphics[width=\linewidth]{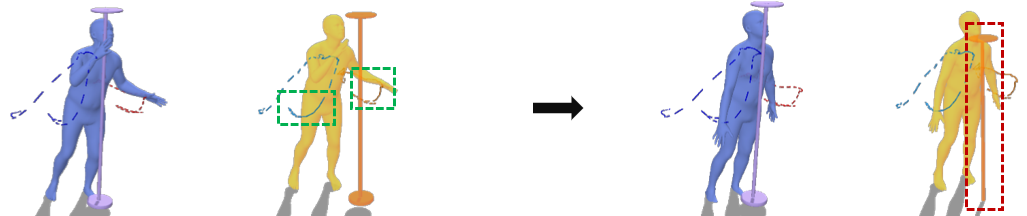}
        \caption{False-positive contact}
        \label{fig:failure_case_b}
    \end{subfigure}
    
    \begin{subfigure}{\columnwidth}
        \centering
        \includegraphics[width=\linewidth]{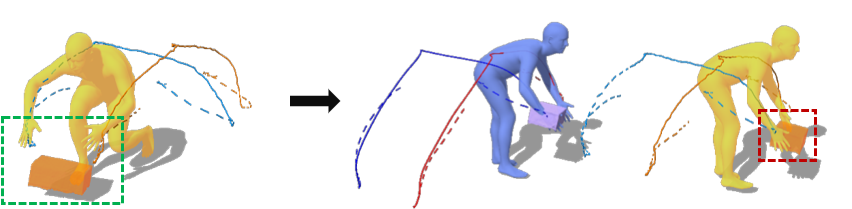}
        \caption{Inaccurate pre-contact hands position}
        \label{fig:failure_case_c}
    \end{subfigure}
    
    \caption{Typical failure cases of our method. Errors in pose or contact estimation can propagate to the final object position.}
    \label{fig:failure_cases}
\end{figure}

\section{Discussion and Limitations}
\label{sec:discussion}

Our work presents a significant step forward in the field of inertial human–object interaction (HOI) estimation by demonstrating that sparse IMUs can be used to capture both human pose and object trajectories in real-world interaction scenarios. This framework is particularly suited for applications where conventional vision-based methods fail due to occlusion, lighting, or constrained environments, such as immersive AR/VR and human-robot collaboration. By enabling interaction estimation using only wearable inertial sensors, IMU-HOI opens up new possibilities for motion capture in settings where cameras are impractical, such as in outdoor, dynamic environments or in applications involving mobile or wearable devices.

Despite these promising advancements, several limitations remain. First, while our method works well for known interactions between the human and a specific object, \textbf{it is inherently limited to scenarios where the object is already instrumented with an IMU}. The ability to generalize this to arbitrary objects or uninstrumented objects remains a significant challenge, as our approach currently relies on knowing the object’s IMU readings and the precise hand-object contact. Additionally, in scenarios involving multiple interacting objects, our current model struggles with accurately estimating the interaction dynamics between the human and other parts of the body (e.g., feet or torso) and the object, which could lead to errors in object tracking and hand-object interaction accuracy.

\textbf{Another limitation arises when handling long sequences.} While our method performs well on shorter, dynamic interactions, longer sequences are prone to drift over time due to the accumulating errors from inertial integration, particularly for object trajectories. The lack of visual cues for continuous error correction exacerbates this issue. Moreover, in some complex interactions where the object slides or rotates relative to the hand, or when there are multiple contact points between the body and object, the model’s assumptions (e.g., single contact point and quasi-rigid object motion) break down, leading to degraded performance. Similarly, estimating the object motion during free movement (without continuous contact) can be prone to drift and inaccuracies, as the reliance on inertial signals alone is insufficient to resolve all ambiguities.

We further analyze several representative failure cases of our pipeline. Since the third-stage object position estimation depends on the outputs of human pose estimation and contact estimation, errors in these earlier stages can directly propagate to the final object trajectory. We identify three common failure modes: (i) missed contact, where actual contact is not detected (Fig.~\ref{fig:failure_case_a}) ; (ii) false-positive contact, where contact is predicted despite the absence of physical interaction (Fig.~\ref{fig:failure_case_b}) ; and (iii) inaccurate pre-contact hand pose, where the contact state is correct but the estimated hand position before contact is erroneous (Fig.~\ref{fig:failure_case_c}) . The first two failure modes are likely related to noise in the human or object IMUs, as well as accumulated velocity errors that impair reliable contact inference. The third arises from the lack of an object mesh, which prevents explicitly constraining or correcting the hand to lie on the object surface. All of these errors can ultimately lead to noticeable drifts in the estimated object position.

\textbf{Lastly, the diversity of objects presents another challenge.} Our method has been evaluated with a fixed set of objects, but real-world applications would involve a much broader range of objects with varying shapes, sizes, and materials. The lack of detailed object models or hand observations limits the system’s ability to handle the full range of interactions, especially with deformable objects or objects with complex shapes. Without visual cues or object meshes, fine-grained interactions, such as nuanced hand-object poses or multi-object interactions, are difficult to estimate with high accuracy.

Despite these limitations, IMU-HOI represents a promising approach to robust and scalable human-object interaction estimation, providing new avenues for motion capture in real-world applications. Future work will aim to address these challenges by incorporating multi-modal sensing (Ego-image), improving the handling of long sequences, and expanding the model’s ability to deal with a wider variety of objects and interaction types.
